# Supplementary material for: Damage-cluster distributions and size effect on strength in compressive failure
Source: arXiv:1203.0850 source file (2012-05-02)
Supplement: Supplementary file 1 [file LM13290_supp_mat.pdf]

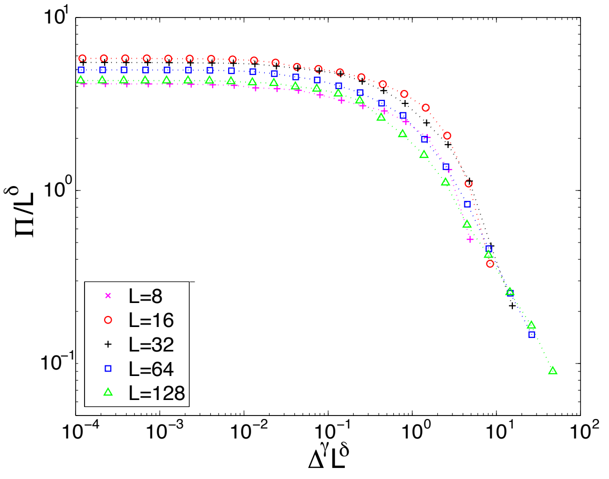


FIG. I. Finite size effect analysed from the growth of the largest damage cluster size $\Pi$ in the pre-peak load phase. $\Pi$ is equivalent to the high-order moment of the distribution of $A$, e.g. $\Pi \sim \langle A^q \rangle^{1/q}$ for $q \to \infty$. Assuming that the size of damage clusters follows a gamma distribution as argued earlier, one can demonstrate that $\Pi \sim A^*$. We hypothesize that for an infinitely large system $\Pi$ diverges as approaching failure ($\Pi(\Delta, L \to \infty) \sim \Delta^\gamma$), whereas for finite size systems it is bounded by a size effect (e.g. $\Pi(\Delta \to 0, L) \sim L^\delta$). The combination of these two effects can be modeled as $\Pi \sim \frac{L^\delta}{L^\delta \Delta^\gamma + c}$, where $c$ is a constant. We test this hypothesis by plotting $\Pi/L^\delta$ vs. $\Delta^\gamma L^\delta$ for all system sizes. Data collapse is obtained for $\delta = 0.3$ for H1, $\delta = 0.8$ for H2 (shown here).

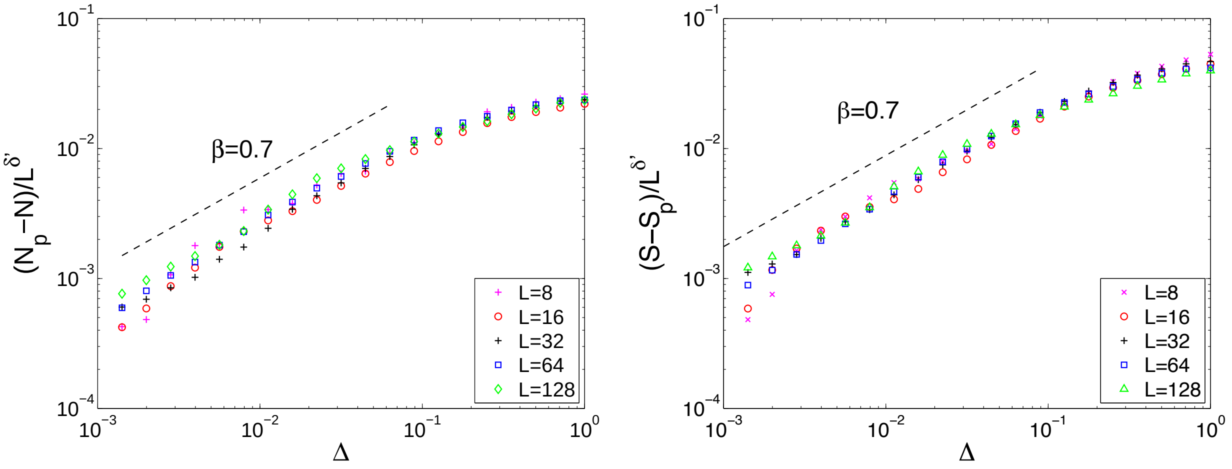


(a) (b)

FIG. II. In the post-peak phase, (a) the number of damage cluster $N$ decreases (i.e. coalescence) following a similar relation as the order parameter $\Pi$: $(N_p - N) \sim L^{\delta'}\Delta^{\beta}$, where $N_p$ is the number of clusters at peak load. (b) The same relation also applies to the increase of the total surface area covered by the damage clusters $S$: $(S - S_p) \sim L^{\delta'}\Delta^{\beta}$, where $S_p$ is the peak load value. The data collapses yield similar exponents as for the order parameter: $\delta' = 1.9$ and $\beta = 0.7$ for H2 disorder.

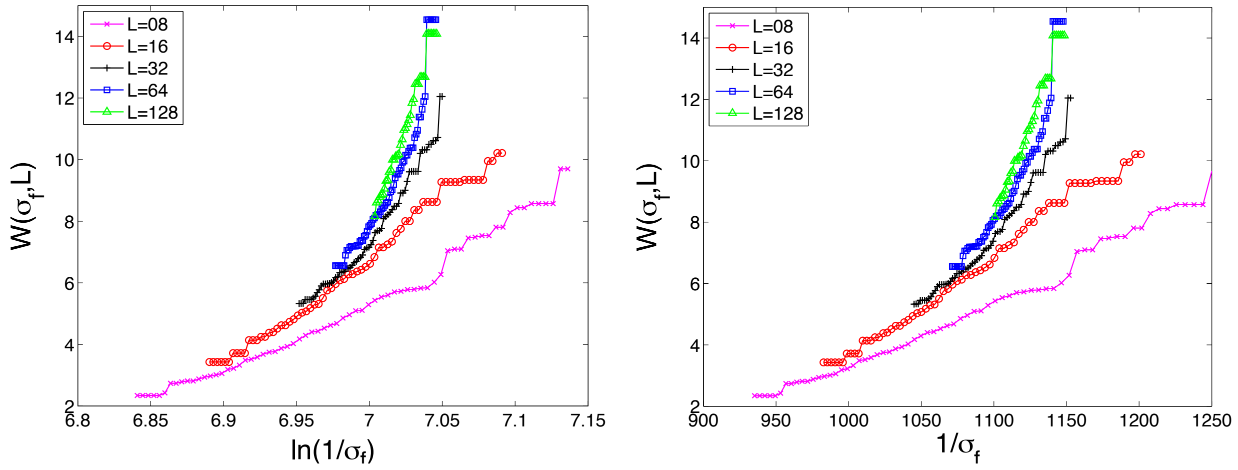


(a) (b)

FIG. III. Probability distribution fits for the failure strength $\sigma_f$ for (a) Weibull distribution, (b) Gumbel distribution, where $W(\sigma_f, L) = -ln\left[-\frac{ln(1-P(\sigma_f))}{L^2}\right]$, $P(\sigma_f)$ is the cumulative probability function. Since the data for different system sizes do not collapse onto a single straight line these distributions are not adequate fits for representing compressive failure strength.
